# Supplementary material for: Constraint-Conditioned Policy Optimization for Versatile Safe Reinforcement Learning
Source: arXiv:2310.03718 source file (2024-04-29)
Supplement: Supplementary file 1 [file appendix-discussion.tex]

\section{Supplementary propositions}
\label{section: supplementary propositions}
\subsection{Optimality guarantee}
The optimality guarantee is mainly derived from the EM-style safe RL training framework, and more details could be found in Appendix A.5 in~\cite{liu2022constrained}. For self-contained, we briefly introduce it as follows.
\begin{Assumption}[Slater's condition]
There exists a feasible distribution $\Bar{q} \in \Pi_\Qcal^{\epsilon_i}$ within the trust region of the old policy $\pi_{\theta_j}(\cdot | \epsilon_i)$: $\KL(\Bar{q}\Vert \pi_{\theta_j}(\cdot | \epsilon_i)) < \kappa, \forall \epsilon_i \in \Ecal$.
\label{assumption:slater}
\end{Assumption}

\begin{Assumption}[Two-step Slater's condition]
\label{assumption:two_e_step}
The Slater's condition holds for both $\pi_{\theta_{j-1}}$ and $\pi_{\theta_j}$.
\end{Assumption}

The above assumptions indicate a well-optimized policy in the constraint-conditioned M-step. In addition, they ensure the variational distributions $q_{j-1}(\cdot | \epsilon_i)$ and $q_{j}(\cdot | \epsilon_i)$ are feasible. Note that an infeasible variational distribution $q_{j-1}(\cdot | \epsilon_i)$ may lead to arbitrarily high reward return. With this assumption, we separately prove the ELBO improvement for constraint-conditioned E-step and versatile M-step.

\begin{Proposition}[Optimality guarantee]
  Suppose the optimal distribution at $j-1$-th and $j$-th update $\pi_{\theta_{j-1}}, \pi_{\theta_{j}}$ both satisfy the Slater's condition, then the ELBO in Eq. (\ref{eq:elbo_new}) is guaranteed to be non-decreasing: $\Jcal(q_j, \theta_{j+1} | \epsilon_i)\geq \Jcal(q_{j-1}, \theta_{j} | \epsilon_i)$.
\label{Proposition:improvement}
\end{Proposition}

\begin{proof}
\textbf{Constraint-conditioned E-step}: By the definition of constrained-condition E-step, we improve the ELBO w.r.t $q(\cdot | \epsilon_i)$. Since $q_{j-1}(\cdot | \epsilon_i)$ is feasible (reward return is bounded) and $\pi_{\theta_j}(\cdot | \epsilon_i)$ satisfies Slater's condition, we can prove the closed-form solution of the constrain-conditioned E-step update will increase ELBO as shown in Appendix.~\ref{app_subsection: Proof of the closed-form solution}: 
$$
\begin{aligned}
&\begin{cases}
\begin{aligned}
q_{j}(\cdot | \epsilon_i) &= \argmax_{q\in \Pi_{\Qcal}^{\epsilon_i}} \mathbb{E}_{\rho_q}\left[\mathbb{E}_{a\sim q(\cdot|s, \epsilon_i)} \left[ \hat{Q}^{\pi_{\theta_j}}_r(s,a | \epsilon_i)\right] - \alpha \KL[q(\cdot|s, \epsilon_i) \| \pi_{\theta_i}(\cdot|s, \epsilon_i)] \right]   \\
&= \argmax_{q\in \Pi_{\Qcal}^{\epsilon_i}} \mathbb{E}_{\tau\sim q} \left[ \sum_{t=0}^\infty \left(\gamma^t r_t - \alpha\KL(q(\cdot| s_t, \epsilon_i)  \| \pi_{\theta_j}(\cdot|s_t, \epsilon_i))\right)\right]\\
&= \argmax_{q\in \Pi_{\Qcal}^{\epsilon_i}} \Jcal(q,\theta_j | \epsilon_i)
\end{aligned}\\
q_{i-1}(\cdot | \epsilon_i) \in \Pi_{\Qcal}^{\epsilon_i}
\end{cases}\\
\Rightarrow & \Jcal(q_j,\theta_j | \epsilon_i) \geq \Jcal(q_{j-1},\theta_j | \epsilon_i).
\end{aligned}
$$
Therefore, as long as assumption \ref{assumption:two_e_step} holds, the ELBO will increase monotonically in terms of $q$.

\textbf{Versatile M-step}: Assuming the ELBO conditioned on different constraints $\epsilon_i \in \Ecal$ are independent of $\theta$. By definition in Eq.~(\ref{eq:mstep}), when conditioned on $\epsilon_i$, we update $\theta$ by
$$
\begin{aligned}
\theta_{j+1} &= \argmax_{\theta} \mathbb{E}_{\rho_{q_j}}\left[\alpha \mathbb{E}_{a\sim q_j(\cdot|s, \epsilon_i)} \left[ \log \pi_\theta (a|s, \epsilon_i)\right]\right] + \log p(\theta) \\
&= \argmax_{\theta} \mathbb{E}_{\rho_{q_j}}\left[- \alpha\KL[q_i(\cdot| s_t, \epsilon_i)  \Vert \pi_\theta(\cdot|s, \epsilon_i)]\right] + \log p(\theta) \\
&= \argmax_{\theta} \mathbb{E}_{\rho_{q_j}} \left[ \mathbb{E}_{a\sim q_j(\cdot|s, \epsilon_j)} \big[ \hat{Q}_r^{q_j}(s,a|\epsilon_i)\big] - \alpha\KL[q_j(\cdot| s_t, \epsilon_i)  \Vert \pi_\theta(\cdot|s, \epsilon_i)]\right] + \log p(\theta)\\
&= \argmax_{\theta} \Jcal(q_j, \pi_{\theta} | \epsilon_i).
\end{aligned}
$$
Therefore, we have:
$
\Jcal(q_j, \pi_{\theta_{j+1}} | \epsilon_i) \geq \Jcal(q_{j}, \pi_{\theta_{j}} | \epsilon_i) 
$. 
Combining all the above together, we have
$$
\Jcal(q_i, \pi_{\theta_{j+1}} | \epsilon_i) \geq \Jcal(q_{i}, \pi_{\theta_{j}}| \epsilon_i) \geq \Jcal(q_{i-1}, \pi_{\theta_{j}}| \epsilon_i) .
$$
\end{proof}

\subsection{Training robustness}
The training robustness is mainly derived from the EM-style safe RL training framework, and more details could be found in Appendix A.6 in~\cite{liu2022constrained}. For self-contained, we briefly introduce it as follows.
\begin{Proposition}[Training robustness]
  Suppose $\pi_{\theta_{j}}(\cdot | \epsilon_i) \in \Pi_\Qcal^{\epsilon_i}$. $\pi_{\theta_{j+1}}$ and $\pi_{\theta_{j}}$ are related by the M-step. If $\epsilon_i < \gamma$, where $\epsilon_i, \gamma$ are the KL threshold in constraint-conditioned E-step and versatile M-step respectively, then the variational distribution $q_{j+1}^*$ in the next iteration is guaranteed to be feasible and optimal.
\label{Proposition:robustness_gurantee}
\end{Proposition}
\begin{proof}
Since $\epsilon < \epsilon_2$, the KL divergence between $\pi_{\theta_{i+1}}$ and $\pi_{\theta_i}$ $\KL(\pi_{\theta_{i}} \Vert \pi_{\theta_{i+1}}) \leq \epsilon < \epsilon_2$. Thus, the Slater condition \ref{assumption:slater} holds for $\pi_{\theta_{i+1}}$ as long as $\pi_{\theta_{i}}$ is feasible, because at least one feasible solution $\pi_{\theta_{i}}$ within the trust region exists. In Appendix.~\ref{app_subsection: Proof of the closed-form solution}, we know that $q_{i+1}^*(\cdot | \epsilon_i)$ in the constraint-conditioned E-step is guaranteed to be feasible and optimal.
\end{proof}
