# Supplementary material for: Constraint-Conditioned Policy Optimization for Versatile Safe Reinforcement Learning
Source: arXiv:2310.03718 source file (2024-04-29)
Supplement: Supplementary file 2 [file appendix-experiment.tex]

% \section{Implementation Details}
% \label{app:implementation}
\clearpage
\section{Supplementary experiments}
\label{section: supplementary experiments}

\subsection{Q functions estimation verification}
\label{subsection: Q functions estimation verification}
The verification results for the Q function estimation are shown in Figure.~\ref{fig: Q-verification}. The testing task is \texttt{Car-Circle}, the behavior policy condition set is $\tilde{\Ecal} = \{20, 40, 60\}$, and the evaluating thresholds are set to be $\{10, 20, 30, 40, 50, 60, 70\}$. We select $Q_c$ as the testing Q function. The ``ground truth'' of the Q functions are the Q functions trained with the single-threshold safe RL agents (CVPO~\cite{liu2022constrained}). The state-action pair data $(s, a)$ for evaluation are sampled randomly from the replay buffer of one single-threshold CVPO agent. We can see from Figure.~\ref{fig: Q-verification} that the $Q_c$ distribution mismatch is small on generalized thresholds, which shows that the proposed VVE is efficient in Q function zero-shot adaptation.

\begin{figure}[!ht]
\centering
\includegraphics[width=0.8\linewidth]{Figures/appendix/Q_verification.png}

    \caption{Q function estimation verification. Green histograms represent the evaluation results of the single-threshold policies (``ground truth''), and the blue histograms represent the evaluation results for the versatile Q function.}
    % \vspace{-10pt}
    \label{fig: Q-verification}
\end{figure}

\subsection{Experiment task details}
Due to the page limit, we omit some descriptions of experiments in the main context. Here we give the full details of our experiment settings. The simulation environments are from a publicly available benchmark~\cite{gronauer2022bullet}. We consider two tasks (Run and Circle) and four robots (Ball, Car, Drone, and Ant) which have been used in many previous works as the testing ground \cite{liu2022robustness, liu2023constrained,achiam2017constrained}.
% For the Run task, the agents are rewarded for running fast between two boundaries and are given constraint violation cost if they run across the boundaries or exceed an agent-specific velocity threshold. 
For the Circle task, the agents are rewarded for running in a circle but are constrained within a safe region smaller than the target circle's radius.
We name the tasks as \texttt{Ball-Circle}, \texttt{Car-Circle}, \texttt{Drone-Circle}, \texttt{Drone-Run}, and \texttt{Ant-Run}. In the Run tasks, agents are rewarded for running fast between two safety boundaries and are given costs for violation constraints if they run across the boundaries or exceed an agent-specific velocity threshold.
The reward and cost functions are defined as:
\begin{align*}
    % r(s) & = \sqrt{(x_{t-1}-g_x)^2 + (y_{t-1}-g_y)^2} - \sqrt{(x_t-g_x)^2 + (y_t-g_y)^2} + r_{robot}(s) \\
    r(\bm{s_t}) & = ||\bm{x_{t-1}}-\bm{g}||_2 - ||\bm{x}_t-\bm{g}||_2 + r_{robot}(s_t) \\
    c(\bm{s_t}) & = \bm{1} (|y| > y_{lim}) + \bm{1}(||\bm{v_t}||_2 > v_{lim})
\end{align*}
where $v_{lim}$ is the speed limit, $y_{lim}$ specifies the safety region, $\bm{v_t} = [v_x, v_y]$ is the velocity of the agent at timestamp $t$, $\bm{g}= [g_x, g_y]$ is the position of a fictitious target, $\bm{x_t} = [x_t, y_t]$ is the position of the agent at timestamp $t$, and $r_{robot}(\bm{s_t})$ is the specific reward for different robot. 
For example, an ant robot will gain reward if its feet do not collide with each other. 
In the Circle tasks, the agents are rewarded for running in a circle in a clockwise direction but are constrained to stay within a safe region that is smaller than the radius of the target circle.
The reward and cost functions are defined as:
\begin{align*}
    r(\bm{s_t}) & = \frac{-y_t v_x + x_t v_y}{1 + | ||\bm{x_t}||_2-r|} + r_{robot}(\bm{s_t}) \\
    c(\bm{s_t}) & = \bm{1}(|x| > x_{lim})
\end{align*}
where $r$ is the radius of the circle, and $x_{lim}$ specifies the range of the safety region.

\subsection{More experiments with different choices of behavior policy conditions}
Due to the page limit, we only provide the experiment results based on behavior policy set $\Ecal = \{20, 40, 60\}$. Here we provide more experiment results when the behavior policy set is selected to be $\tilde{\Ecal} = \{10, 30, 50, 70\}$ as shown in Table.~\ref{tab: more_bp}. The algorithms are evaluated on threshold conditions $\Ecal = \{10, 15, ..., 70\}$ for the \texttt{Ball-Circle}, \texttt{Car-Circle}, and \texttt{Drone-Circle} tasks. From the results, we can clearly see that all the conclusions in section~\ref{subsection: Main Results and Analysis} also hold for different behavior policy choices.

% Table generated by Excel2LaTeX from sheet 'Sheet1'
\begin{table}[htbp]
  \centering
  \vspace{-5pt}
  \caption{Evaluation results of proposed CCPO method and the proposed versatile safe RL baselines. $\uparrow$: the higher reward, the better. $\downarrow$: the lower constraint violation (minimal 0), the better. The models are evaluated on a series of threshold conditions and we report the averaged reward and constraint violation values on all evaluation thresholds and generalized thresholds. Each value is reported as mean ± standard deviation for 50 episodes and 5 seeds. We shade the two safest agents with the lowest averaged cost violation values.}
  \vspace{5pt}
  \scriptsize
    \begin{tabular}{ccccccc}
    \toprule
    \multirow{2}[4]{*}{Task} & \multirow{2}[4]{*}{Stats} & \multirow{2}[4]{*}{CCPO (ours)} & \multicolumn{2}{c}{Constraint-conditioned} & \multicolumn{2}{c}{Linear combination} \\
\cmidrule{4-7}          &       &       & V-SAC-Lag & V-DDPG-Lag & C-PPO-Lag & C-TRPO-Lag \\
    \midrule
    \multirow{4}[2]{*}{Ball-Circle} & Avg. R $\uparrow$ & \cellcolor[rgb]{ .906,  .902,  .902}639.65±37.91 & 778.14±7.92 & 737.79±29.84 & \cellcolor[rgb]{ .906,  .902,  .902}590.58±20.76 & 700.86±2.81 \\
          & Avg. CV & \cellcolor[rgb]{ .906,  .902,  .902}0±0 & 5.98±2.29 & 2.36±1.30 & \cellcolor[rgb]{ .906,  .902,  .902}0.84±0.58 & 1.78±0.36 \\
          & Avg. R-G $\uparrow$ & \cellcolor[rgb]{ .906,  .902,  .902}640.71±37.46 & 781.82±7.73 & 739.22±28.98 & \cellcolor[rgb]{ .906,  .902,  .902}589.08±18.85 & 702.74±2.93 \\
          & Avg. CV-G & \cellcolor[rgb]{ .906,  .902,  .902}0±0 & 5.95±2.06 & 2.64±1.45 & \cellcolor[rgb]{ .906,  .902,  .902}0.56±0.48 & 2.28±0.40 \\
    \midrule
    \multirow{4}[2]{*}{Car-Circle} & Avg. R $\uparrow$ & \cellcolor[rgb]{ .906,  .902,  .902}414.08±3.47 & 342.68±12.59 & 436.02±33.56 & 440.31±9.83 & \cellcolor[rgb]{ .906,  .902,  .902}457.25±1.29 \\
          & Avg. CV $\downarrow$ & \cellcolor[rgb]{ .906,  .902,  .902}1.18±0.36 & 14.18±6.24 & 19.60±13.67 & 9.49±1.47 & \cellcolor[rgb]{ .906,  .902,  .902}8.63±1.38 \\
          & Avg. R-G $\uparrow$ & \cellcolor[rgb]{ .906,  .902,  .902}414.36±3.17 & 344.02±13.38 & 436.72±33.92 & \cellcolor[rgb]{ .906,  .902,  .902}441.92±9.16 & 456.23±2.16 \\
          & Avg. CV-G $\downarrow$ & \cellcolor[rgb]{ .906,  .902,  .902}1.19±0.35 & 15.23±7.27 & 21.06±14.91 & \cellcolor[rgb]{ .906,  .902,  .902}11.05±1.82 & 11.24±1.02 \\
    \midrule
    \multirow{4}[2]{*}{Drone-Circle} & Avg. R $\uparrow$ & \cellcolor[rgb]{ .906,  .902,  .902}703.06±31.82 & 696.92±35.98 & 719.54±95.85 & \cellcolor[rgb]{ .906,  .902,  .902}367.84±15.85 & 489.42±9.40 \\
          & Avg. CV $\downarrow$ & \cellcolor[rgb]{ .906,  .902,  .902}0±0 & 5.39±4.45 & 11.06±10.12 & \cellcolor[rgb]{ .906,  .902,  .902}2.09±1.62 & 8.64±1.42 \\
          & Avg. R-G $\uparrow$ & \cellcolor[rgb]{ .906,  .902,  .902}705.52±30.35 & 702.72±36.73 & 721.57±95.17 & \cellcolor[rgb]{ .906,  .902,  .902}277.42±19.26 & 427.59±10.26 \\
          & Avg. CV-G $\downarrow$ & \cellcolor[rgb]{ .906,  .902,  .902}0±0 & 5.92±5.03 & 11.37±10.78 & \cellcolor[rgb]{ .906,  .902,  .902}2.82±1.94 & 12.05±1.74 \\
    \bottomrule
    \end{tabular}%
  \label{tab: more_bp}%
\end{table}%

\subsection{More baseline comparison experiments}
We also compare our method with C-CPO, which is modified from CPO with the policy linear combination. The comparison results are shown in Table. \ref{tab: CPO baseline}. It is evident that the proposed CCPO method outperforms Versatile CPO in terms of both constraint satisfaction and reward efficiency.

% Table generated by Excel2LaTeX from sheet 'Sheet1'
\begin{table}[htbp]
  \centering
  \caption{\small C-CPO baseline comparison}
  \scriptsize
    \begin{tabular}{cccccccc}
    \toprule
    Tasks & stats & BC    & CC    & DC    & DR    & AR    & Average \\
    \midrule
          & Avg. R & \textcolor[rgb]{ .2,  .2,  .2}{686.08 ± 2.58} & \textcolor[rgb]{ .2,  .2,  .2}{455.87 ± 1.51} & \textcolor[rgb]{ .2,  .2,  .2}{565.98 ± 5.71} & \textcolor[rgb]{ .2,  .2,  .2}{304.09 ± 32.17} & \textcolor[rgb]{ .2,  .2,  .2}{602.05 ± 1.66} & \textcolor[rgb]{ .2,  .2,  .2}{522.81} \\
    C-CPO & Avg. CV & \textcolor[rgb]{ .2,  .2,  .2}{1.77 ± 0.67} & \textcolor[rgb]{ .2,  .2,  .2}{4.50 ± 2.08} & \textcolor[rgb]{ .2,  .2,  .2}{6.32 ± 2.32} & \textcolor[rgb]{ .2,  .2,  .2}{11.82 ± 5.85} & \textcolor[rgb]{ .2,  .2,  .2}{2.19 ± 0.63} & \textcolor[rgb]{ .2,  .2,  .2}{6.6} \\
          & Avg. R-G & \textcolor[rgb]{ .2,  .2,  .2}{676.27 ± 2.32} & \textcolor[rgb]{ .2,  .2,  .2}{454.62 ± 1.97} & \textcolor[rgb]{ .2,  .2,  .2}{559.71 ± 7.32} & \textcolor[rgb]{ .2,  .2,  .2}{300.85 ± 32.41} & \textcolor[rgb]{ .2,  .2,  .2}{592.89 ± 2.68} & \textcolor[rgb]{ .2,  .2,  .2}{516.87} \\
          & Avg. CV-G & \textcolor[rgb]{ .2,  .2,  .2}{2.09 ± 0.59} & \textcolor[rgb]{ .2,  .2,  .2}{4.94 ± 2.37} & \textcolor[rgb]{ .2,  .2,  .2}{6.75 ± 2.47} & \textcolor[rgb]{ .2,  .2,  .2}{13.07 ± 5.44} & \textcolor[rgb]{ .2,  .2,  .2}{2.28 ± 0.73} & \textcolor[rgb]{ .2,  .2,  .2}{5.83} \\
    \midrule
          & Avg. R & \textcolor[rgb]{ .2,  .2,  .2}{710.86 ± 20.47} & \textcolor[rgb]{ .2,  .2,  .2}{406.06 ± 6.30} & \textcolor[rgb]{ .2,  .2,  .2}{630.55 ± 40.03} & \textcolor[rgb]{ .2,  .2,  .2}{458.69 ± 12.98} & \textcolor[rgb]{ .2,  .2,  .2}{660.88 ± 4.82} & \textcolor[rgb]{ .173,  .227,  .29}{\textbf{573.41}} \\
    CCPO  & Avg. CV & \textcolor[rgb]{ .2,  .2,  .2}{0.59 ± 0.31} & \textcolor[rgb]{ .2,  .2,  .2}{1.60 ± 0.91} & \textcolor[rgb]{ .2,  .2,  .2}{0.32 ± 0.38} & \textcolor[rgb]{ .2,  .2,  .2}{0.23 ± 0.25} & \textcolor[rgb]{ .2,  .2,  .2}{3.13 ± 1.67} & \textcolor[rgb]{ .173,  .227,  .29}{\textbf{1.17}} \\
          & Avg. R-G & \textcolor[rgb]{ .2,  .2,  .2}{699.04 ± 20.48} & \textcolor[rgb]{ .2,  .2,  .2}{401.53 ± 5.59} & \textcolor[rgb]{ .2,  .2,  .2}{625.51 ± 40.12} & \textcolor[rgb]{ .2,  .2,  .2}{455.64 ± 11.83} & \textcolor[rgb]{ .2,  .2,  .2}{660.07 ± 5.26} & \textcolor[rgb]{ .173,  .227,  .29}{\textbf{568.36}} \\
          & Avg. CV-G & \textcolor[rgb]{ .2,  .2,  .2}{0.83 ± 0.42} & \textcolor[rgb]{ .2,  .2,  .2}{1.49 ± 0.38} & \textcolor[rgb]{ .2,  .2,  .2}{0.47 ± 0.55} & \textcolor[rgb]{ .2,  .2,  .2}{0.33 ± 0.37} & \textcolor[rgb]{ .2,  .2,  .2}{3.25 ± 1.48} & \textcolor[rgb]{ .173,  .227,  .29}{\textbf{1.27}} \\
    \bottomrule
    \end{tabular}%
  \label{tab: CPO baseline}%
\end{table}%
