# Supplementary material for: Constraint-Conditioned Policy Optimization for Versatile Safe Reinforcement Learning
Source: arXiv:2310.03718 source file (2024-04-29)
Supplement: Supplementary file 3 [file appendix-implementation.tex]

\section{Implementation details}
\label{section: CCPO implementation details}
\subsection{CCPO implementation details}
Due to the page limit, we omit the implementation details of CCPO in the main content. We will present the full algorithm and some implementation tricks in this section. Without otherwise statements, the critics' and policies' parametrization is assumed to be neural networks (NNs), while we believe other parametrization forms should also work in practice.

\textbf{Critics update}. Denote $\phi_{\psi_\fs}, \phi_{z_\fs}$ as the parameters for $\psi_\fs(s, a)$ and $z_{\fs}(\epsilon)$ in the critic $Q_\fs(s, a|\epsilon)$. Similar to many other off-policy algorithms~\cite{lillicrap2015continuous}
%~\cite{lillicrap2015continuous}
, we use a target network for each critic and the polyak smoothing trick to stabilize the training. Other off-policy critic's training methods, such as Re-trace
% ~\cite{munos2016safe}
, could also be easily incorporated with the CCPO training framework. Denote $\phi_{\psi_r}^{\prime}, \phi_{z_r}^{\prime}$ as the parameters for the \textbf{target} reward critic $Q_r'$, and $\phi_{\psi_c}^{\prime}, \phi_{z_c}^{\prime}$ as the parameters for the \textbf{target} cost critic $Q_c'$. Define $\Dcal = \cup_{\tilde{\epsilon}_i \in \tilde{\Ecal}} \Dcal_i$ as the replay buffer and $(s, a, s', r, c, \tilde{\epsilon}_i)$ as the state, action, next state, reward, cost, and behavior policy condition, respectively. The critics are updated by minimizing the following mean-squared Bellman error (MSBE):
\begin{align}
  & L(\phi_r) = \sum_{\Dcal_i} \mathbb{E}_{(s, a, s', r, c) \sim \Dcal_i}\Big[\left( Q_r(s, a|\epsilon_i) -  (r + \gamma \mathbb{E}_{a'\sim \pi(\cdot | \epsilon_i)}[ Q_r'(s', a'|\epsilon_i) ] ) \right)^2 \Big]
  \label{eq:qr_loss}\\
  & L(\phi_c) = \sum_{\Dcal_i} \mathbb{E}_{(s, a, s', r, c) \sim \Dcal_i} \Big[\left( Q_c(s, a|\epsilon_i) -  (c + \gamma \mathbb{E}_{a' \sim \pi(\cdot | \epsilon_i)}[ Q_c'(s', a'|\epsilon_i) ] ) \right)^2 \Big].
  \label{eq:qc_loss}
\end{align}

Denote $\alpha_c$ as the critics' learning rate, we have the following updating equations:
\vspace*{-1mm}
\begin{align}
\label{equ: critics update}
    & \phi_{\psi_\fs} \xleftarrow{} \phi_{\psi_\fs} - \alpha_c \nabla_{\phi_r} L(\phi_r), \quad \phi_{z_\fs} \xleftarrow{} \phi_{z_\fs} - \alpha_c \nabla_{\phi_c} L(\phi_c).
\end{align}

\vspace*{-1mm}
We use the polyak averaging trick to update the critics with a weight parameter $\rho \in (0, 1)$:
\vspace*{-1mm}
\begin{equation}
\begin{aligned}
  &\phi_{\psi_\fs}^{\prime} = \rho \phi_{\psi_\fs}^{\prime} + (1-\rho) \phi_{\psi_\fs} \quad \phi_{z_\fs}^{\prime} = \rho \phi_{z_\fs}^{\prime} + (1-\rho) \phi_{z_\fs}.
\end{aligned}
\label{eq:polyak}
\end{equation}

% \textbf{Full Algorithm}. 
% % The CCPO algorithm is shown in Alg.~\ref{alg: CCPO}.
% Note that for off-policy methods, we need to convert the episodic-wise constraint violation threshold to a state-wise threshold for the $Q_c$ functions.
% Denote $T$ as the episode length, the target cost limit for one episode is $\epsilon_i^T$. Denote the discounting factor as $\gamma$. Then, if we assume that at each time step we have an equal probability to violate the constraint, the target constraint value $\epsilon_{i}$ for safety critic $Q_c^{\pi_{\theta_j}}(\cdot | \epsilon_i)$ could be approximated by:
% $$
% \epsilon_{i} =  \epsilon_i^T \times \frac{1-\gamma^T}{T(1-\gamma)}
% $$
% The converted threshold $\epsilon_i$ will be used to compute the Lagrangian multipliers for the baselines, and also be used as one of the constraint thresholds in the constraint-conditioned E-step of our method:
% $$
% \int \pi(a|s, \epsilon_i) \hat{Q}_c^{\pi_{\theta_j}}(s,a|\epsilon_i) \leq \epsilon_{i}, \quad\forall s, a
% $$

\textbf{Model structure.} The versatile critics model $Q_{\fs}(s, a|\epsilon_i) = \psi_{\fs}(s, a)^{\top} z_{\fs}(\epsilon_i)$ is shown in Figure.~\ref{fig: versatile Q}. We set the feature dimension $M=32$, and use an MLP with size [256, 256] to map from the state-action pair to the feature $\psi_{\fs}$. Also, we use an MLP with size [32, 32] to map from $\epsilon$ to $z_{\fs}$. 
For the versatile actor, we provide two options for the model structure. The first one is to direct concat the threshold $\epsilon_i$ into the state: $\bar{s} = [s, \epsilon_i]$ (Con) as shown in Figure.~\ref{fig: versatile actor con}. 
The second one is to use the Multiplicative Interaction (MI) structure inspired by previous works~\cite{de2017modulating, van2016conditional, perez2018film, kumar2019reward}. To give a fair comparison, we use the Con net for both our methods and the baseline. The user may turn on the MI option in the code to get a higher performance of our proposed CCPO method.
\begin{figure}[htbp]
\centering
\begin{minipage}[t]{0.33\textwidth}
\centering
\includegraphics[width=0.976\linewidth]{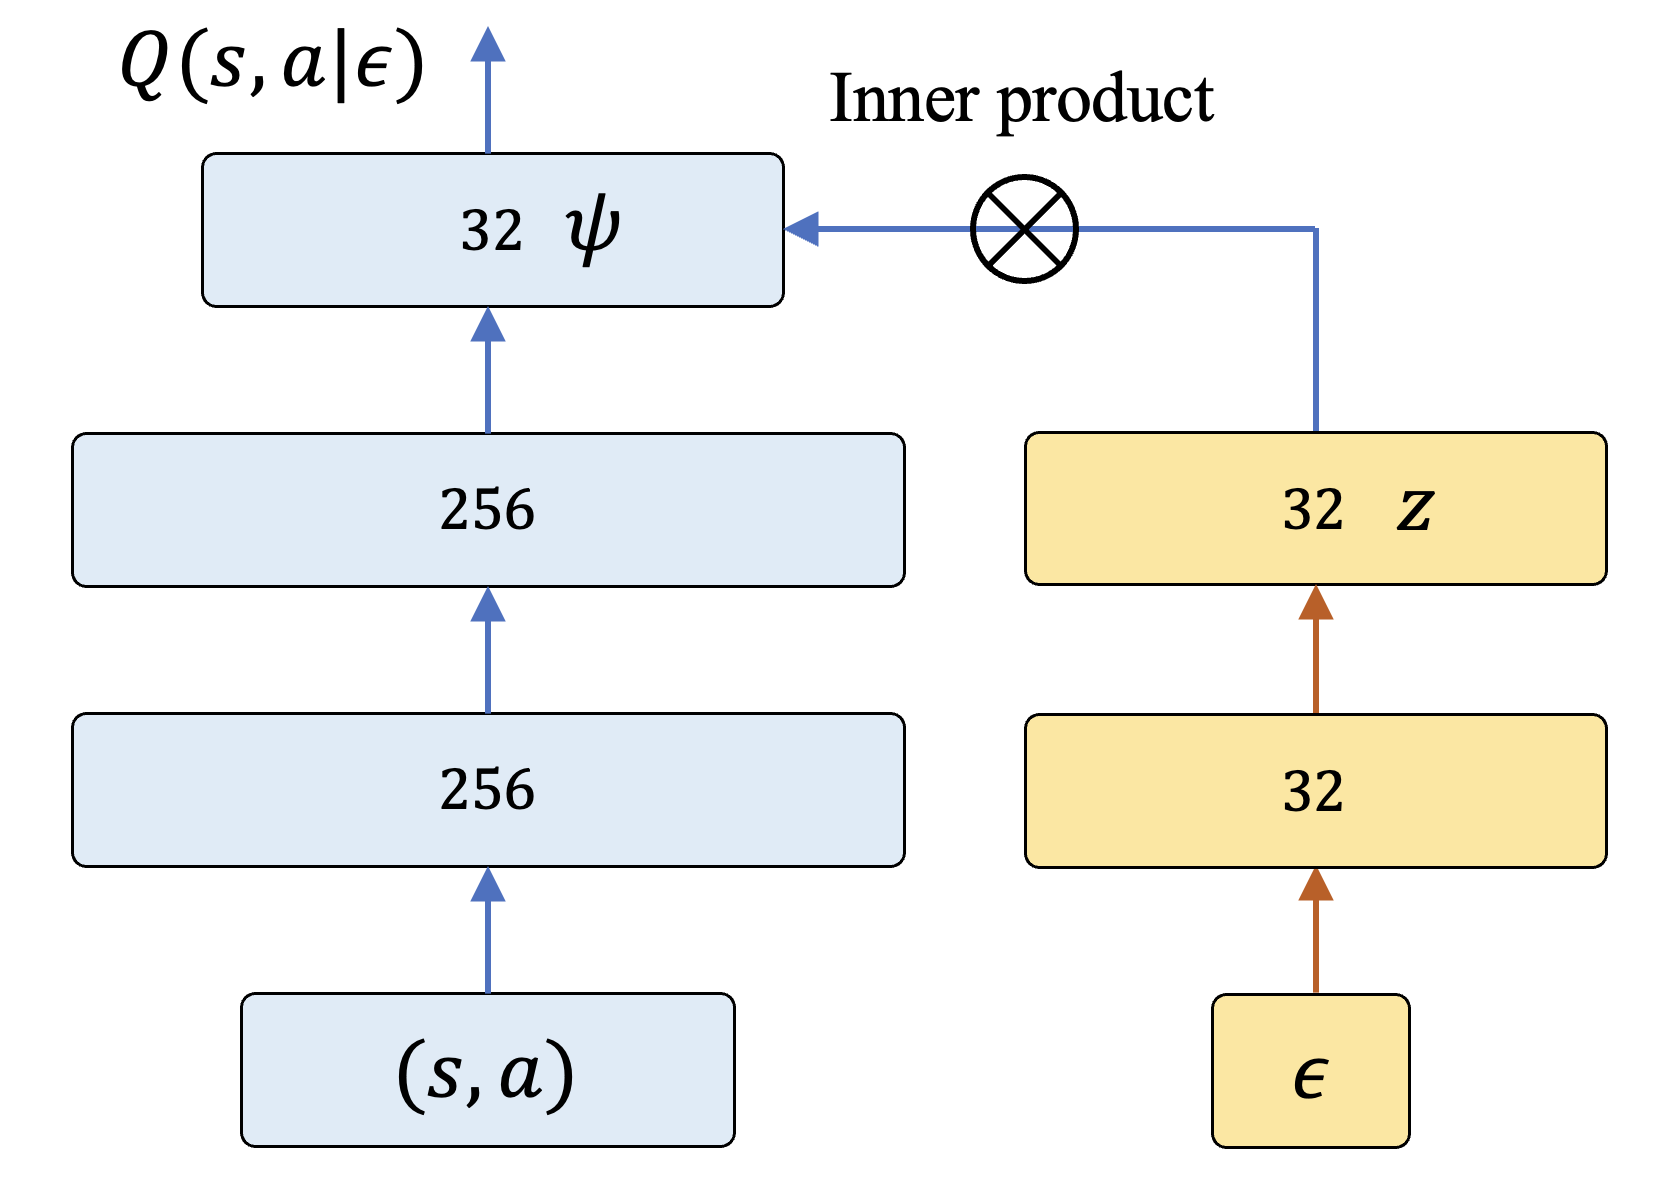}
\caption{Versatile critics using Linear decomposition.}
\label{fig: versatile Q}
\end{minipage}
\ \ 
\begin{minipage}[t]{0.23\textwidth}
\centering
\includegraphics[width=0.78\linewidth]{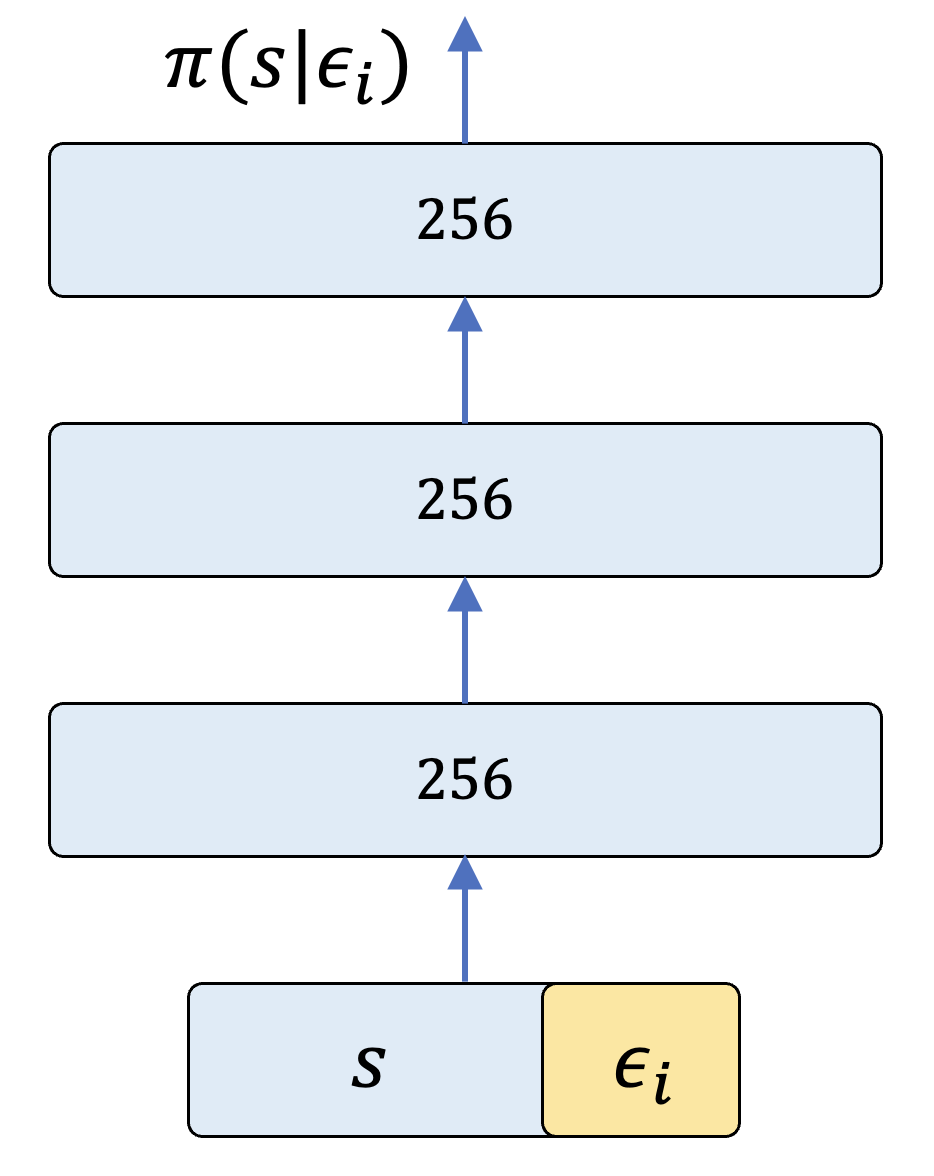}
\caption{Versatile actor using state augmentation.}
\label{fig: versatile actor con}
\end{minipage}
\ \ 
\begin{minipage}[t]{0.4\textwidth}
\centering
\includegraphics[width=\linewidth]{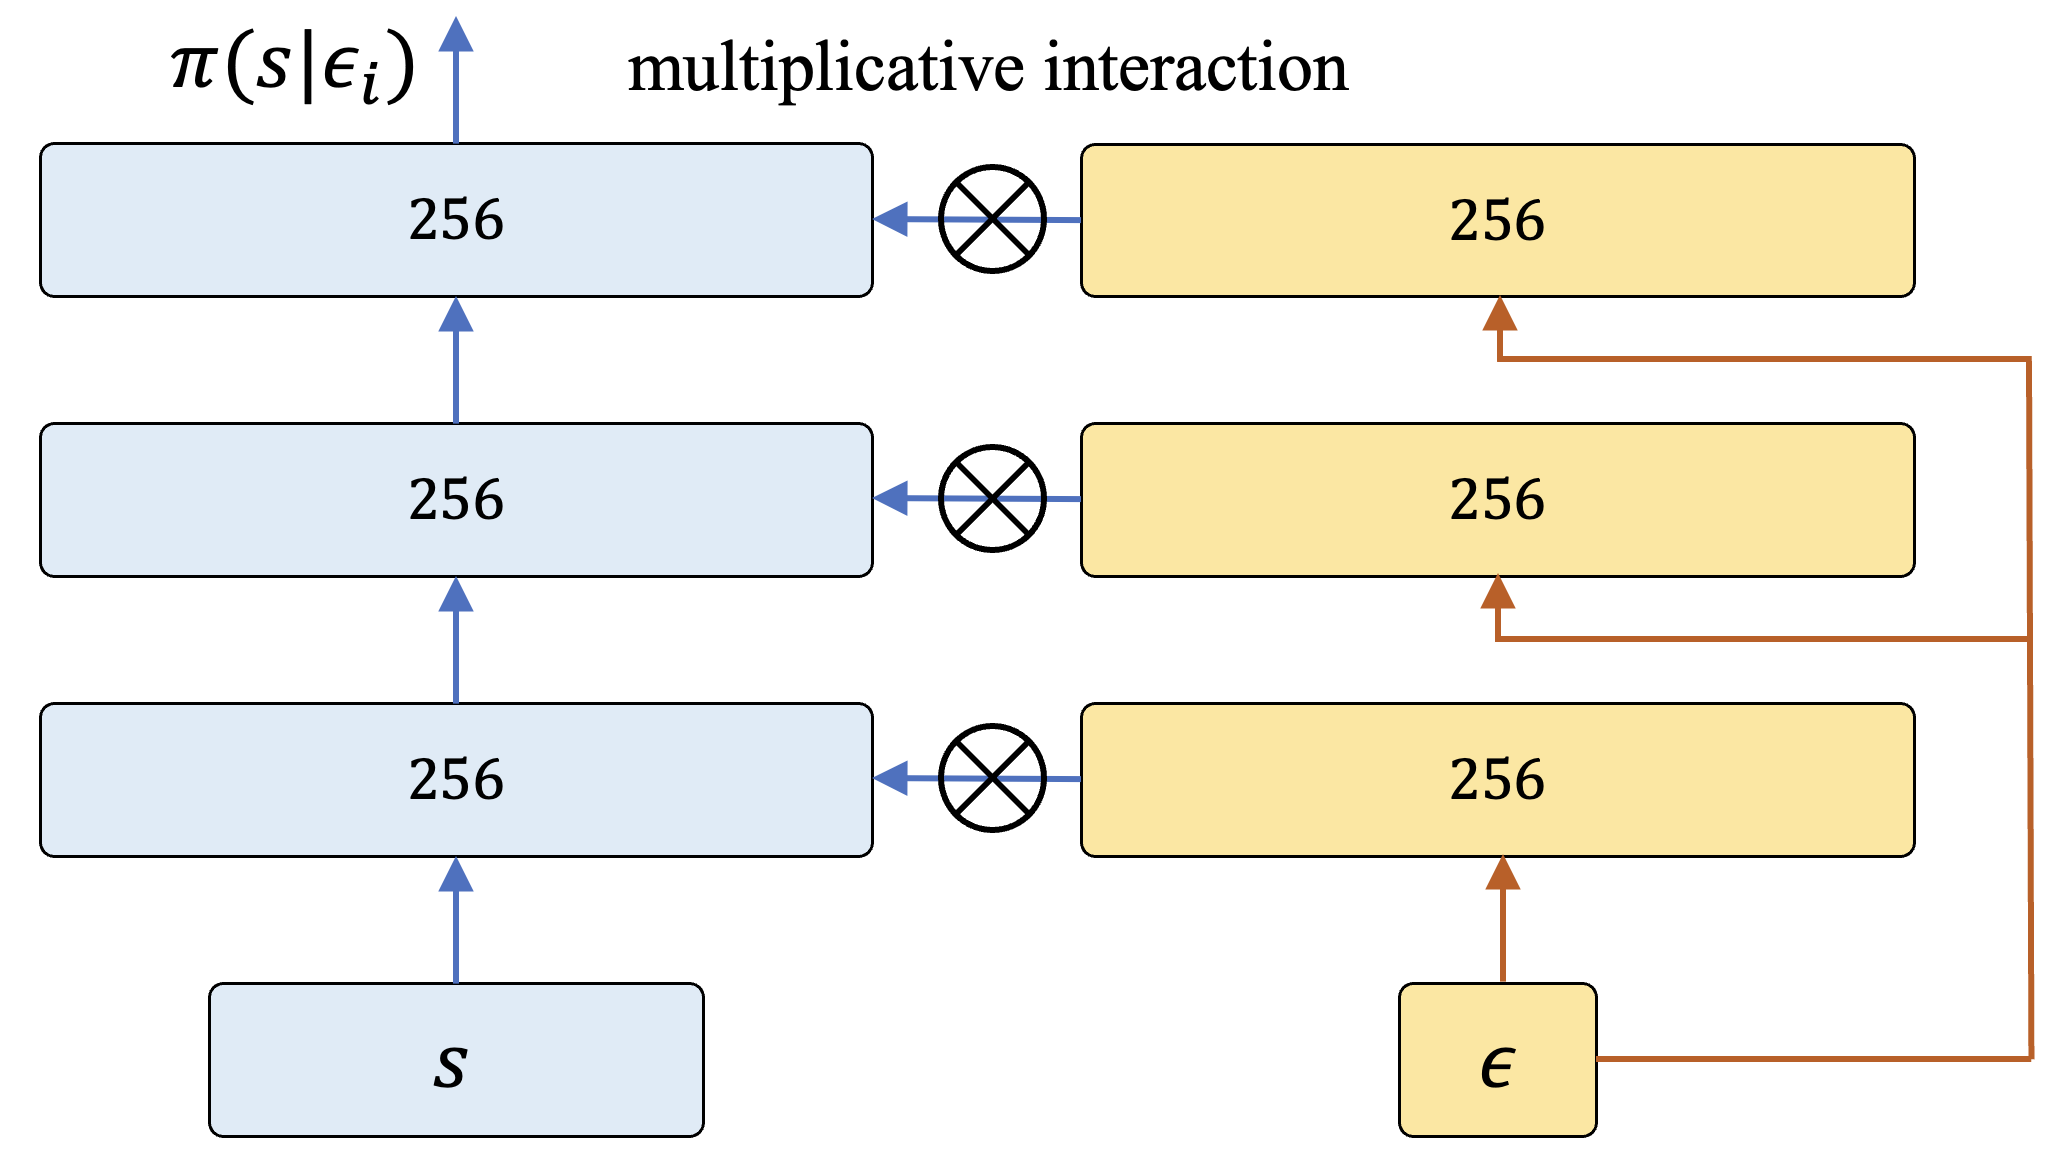}
\caption{Versatile actor using multiplicative interaction.}
\label{fig: versatile actor MI}
\end{minipage}
\end{figure}

\newpage
% \twocolumn

% \begin{algorithm}[h]
% \begin{minipage}[t]{0.55\textwidth}
% \caption{CCPO Training for One Epoch}
% {\bfseries Input:} \raggedright batch size $B$, particle size $K$, policy parameter $\theta_i$ \par
% {\bfseries Output:} \raggedright Updated policy parameter $\theta_{i+1}$ \par
% \begin{algorithmic}[1] % The number tells where the line numbering should start
% \STATE $\triangleright$ \textit{VVE begins}
% \STATE Update $Q_{r}^{\theta_i}(\cdot | \epsilon_i), Q_{c}^{\theta_i}(\cdot | \epsilon)$ for $\epsilon \in \Ecal$ via Bellman backup
% \STATE Sample $B$ transitions from replay buffer
% \STATE $\triangleright$ \textit{Constraint-conditioned E-step begins}
% \STATE Specify $\Ecal_{tra}$ = $\Ecal$ \textbf{if} pre-training \textbf{else} $\tilde{\Ecal}$
% \FOR{$\epsilon_j \in \Ecal_{tra}$}
% \FOR{$b=1,..., B$}
% \STATE Sample $K$ actions $\{a_1,...,a_K\}$ with $\pi^{\theta_i}(\cdot | \epsilon_j)$ for $s_b$
% \STATE Compute $Q_{r}^{\theta_i}(s_b,a_k| \epsilon_j), Q_{c}^{\theta_i}(s_b,a_k| \epsilon_j)$.
% \ENDFOR
% \ENDFOR
% \STATE Compute optimal dual variables $\eta^*(\cdot|\epsilon_j), \lambda^*(\cdot|\epsilon_j)$ by solving the convex optimization problem (10)
% \STATE Compute the optimal variational distribution for each state $\{q^*(\cdot|s_b, \epsilon_j); b=1,...,B\}$ by Eq. (9)
% \STATE $\triangleright$ \textit{Versatile M-step begins}
% \STATE Update policy from $\pi_{\theta_i}$ to $\pi_{\theta_{i+1}}$ via supervised learning objective (12)
% \end{algorithmic} \label{algo:cvpo}
% \end{minipage}
% \end{algorithm}

\onecolumn
