# Supplementary material for: Constraint-Conditioned Policy Optimization for Versatile Safe Reinforcement Learning
Source: arXiv:2310.03718 source file (2024-04-29)
Supplement: Supplementary file 4 [file appendix-proof.tex]

\newpage
\onecolumn

\clearpage
% \appendix
\section{Proofs and discussions}
\label{section: proof and discussions}

\subsection{Proof of Theorem~\ref{Theorem: Bounded estimation error}}
\label{proof: Bounded estimation error}
\begin{proof}
In the proof, we omit the subscript $\fs \in \{r, c\}$ for notation simplicity. The results hold for both cost and reward Q functions.
Denote $\boldsymbol{x_j} = [1, \tilde\epsilon_j, ..., \tilde\epsilon_j^p]$, $\boldsymbol{X}=[\boldsymbol{x_1}^T, ..., \boldsymbol{x_N}^T] \in \R^{(p+1)\times N}$. For each component $z_i$ of $\boldsymbol{z}$, it can be written as:
\begin{equation}
    z^*_i = \boldsymbol{\beta_i}^T \boldsymbol{x} + e_i; \quad i = 1, ..., M
\end{equation}
where $e_i$ is the remainder, and we regard it following the Gaussian distribution: $e_i \sim \Ncal(0, \sigma_i^2)$, and $\sigma_i \leq \sigma$. We divide the proof of the bounded estimation error into the following parts:
    
\textbf{(1) Estimation error bound depending on the threshold $\epsilon$ for generalization:} The objective of the Poly-regression is to find the optimal parameter $\beta_i$ such that it minimizes the Mean Squared Error:
\begin{equation}
    \boldsymbol{\hat{\beta}_i} := \arg \min_\beta \frac{1}{N} \| \boldsymbol{\beta_i}^T  \boldsymbol{X} -\boldsymbol{z}_i \|^2_2
\end{equation}
% \begin{equation}
%     \hat{z}_i = \boldsymbol{\hat{\beta}_i}^T \boldsymbol{x}
% \end{equation}
The point estimation of $\boldsymbol{\beta_i}$ as:
\begin{equation}
    \hat{\boldsymbol{\beta}}_i = \left(\boldsymbol{X}^T \boldsymbol{X}\right)^{-1} \boldsymbol{X}^T \boldsymbol{z}_i
\end{equation}
Without loss of generality, we assume $e_i \sim \Ncal(0, \sigma^2), \forall i$ to derive a loosen bound. In this case, it can be verified that this estimator is unbiased, i.e., 
$\E [ \hat{\boldsymbol{\beta}}_i ] = \boldsymbol{\beta}_i$, and the covariance matrix for $\hat{\boldsymbol{\beta}}_i$ is:
\begin{equation}
    cov(\hat{\boldsymbol{\beta}}_i) = (\boldsymbol{X}^T \boldsymbol{X})^{-1} \boldsymbol{X}^T cov(z_i) \boldsymbol{X} (\boldsymbol{X}^T \boldsymbol{X})^{-1} = \sigma^2 (\boldsymbol{X}^T \boldsymbol{X})^{-1}
\end{equation}
Then the mean of $\psi_{i}(s, a) \hat{z}_i = \psi_{i}(s, a)\boldsymbol{\hat{\beta}_i}^T \boldsymbol{x}$ is:
\begin{equation}
    \E \ \psi_{i}(s, a) \hat{z}_i = \psi_{i}(s, a) \hat{z}^*_i
\end{equation}
and the variance of $\psi_{i}(s, a) \hat{z}_i = \psi_{i}(s, a)\boldsymbol{\hat{\beta}_i}^T \boldsymbol{x}$ is:
\begin{equation}
\begin{aligned}
    \Var(\psi_{i}(s, a)\hat{z}_i)  = \psi_{i}^2(s, a)\boldsymbol{x}^T \Var(\hat{\boldsymbol{\beta}}_i) \boldsymbol{x} = \sigma^2\psi_{i}^2(s, a) \boldsymbol{x}^T (\boldsymbol{X}^T \boldsymbol{X})^{-1} \boldsymbol{x}
\end{aligned}
\end{equation}
Then $\psi_{i}(s, a)\hat{z}_i$ follows the Gaussian distribution:
\begin{equation}
    \psi_{i}(s, a)\hat{z}_i \sim \Ncal(\psi_{i}(s, a) \hat{z}^*_i, \sigma^2\psi_{i}^2(s, a) \boldsymbol{x}^T (\boldsymbol{X}^T \boldsymbol{X})^{-1} \boldsymbol{x})
\end{equation}
Assuming $\hat{z}_i$ are independent of each other, we can get the estimation error of the versatile Q function as:
\begin{equation}
\label{equ: gaussian bound}
    w := \hat{Q}(s, a|\epsilon) - Q^*(s, a|\epsilon) \sim \Ncal\left(0, \sum_{i=1}^{M} \sigma^2\psi_{i}^2(s, a) \boldsymbol{x}^T (\boldsymbol{X}^T \boldsymbol{X})^{-1} \boldsymbol{x}\right)
\end{equation}
% By Gauss-Markov Theorem, $\hat{Q}(s, a|\epsilon)$ is an unbiased and variance-minimizing estimator of ${Q}^*(s, a|\epsilon)$. 
With~(\ref{equ: gaussian bound}), we can get the prediction error bound as:
\begin{equation}
\label{equ: gaussian prediction interval}
    \Pr \left( -z_{{\alpha} / {2}} \leq \frac{\hat{Q}(s, a|\epsilon) - Q^*(s, a|\epsilon)}{ \sqrt{\sum_{i=1}^{M} \sigma^2\psi_{i}^2(s, a) \boldsymbol{x}^T (\boldsymbol{X}^T \boldsymbol{X})^{-1} \boldsymbol{x}} } \leq z_{{\alpha} / {2}} \right) = 1 - \alpha 
\end{equation}
Also since $||\psi_{\fs, i}(s, a)|| \leq K_\fs$, with confidence level $1-\alpha$, we can get:
\begin{equation}
\label{equ: error bound depending on x}
    ||\hat{Q}(s, a|\epsilon) - Q^*(s, a|\epsilon)|| \leq z_{\alpha/2} \sqrt{ \sigma^2 \ M K^2 \boldsymbol{x}^T (\boldsymbol{X}^T \boldsymbol{X})^{-1} \boldsymbol{x}},
\end{equation}
where $z_{\alpha/2}$ is the Z-score for the standard Gaussian distributions. Bound shown in~(\ref{equ: error bound depending on x}) depends on the choice of behavior policy conditions (encoded in $\boldsymbol{X}^T \boldsymbol{X}$) and the targeted threshold for adaptation (encoded in $\boldsymbol{x}$).

\textbf{(2) Upper bound for all the threshold conditions:} In the next, we are going to find the upper bound for $\sqrt{\boldsymbol{x}^T (\boldsymbol{X}^T \boldsymbol{X})^{-1} \boldsymbol{x}}$ to derive an upper bound for any threshold $\epsilon$. First, we assume the threshold conditions for behavior policies are selected to divide the target condition interval $[\epsilon_L, \epsilon_H]$ evenly. We then show that given limited $N \leq N_{max}$, there exists $B_0(p)$ and $\beta_0(p)$ such that the estimation error bound can be presented as:
\begin{equation}
\label{equ: representation assumption}
    ||\hat{Q}(s, a|\epsilon) - Q^*(s, a|\epsilon)|| \leq \frac{B_0(p)}{N^{\beta_0(p)}}
\end{equation}
This result naturally holds since $\boldsymbol{\psi}(s, a)$ is bounded, and $z^*$ can be represented as a polynomial of normalized $\epsilon \in [0, 1]$ (Note that we have normalized the threshold conditions $\epsilon \in [\epsilon_L, \epsilon_H]$ to the interval $[0, 1]$ by $\epsilon = (\epsilon - \epsilon_L) / \epsilon_H$ for numerical stability). One trivial solution is a large enough $B(p)$ and $\beta(p)=0$. The problem is how can we find the tight estimate of $B(p)$ and $\beta(p)$. Here we use the numerical method to find the tight mappings from $p$ to $C$ and $\beta$. When $N \leq 20$, the results are shown as:
\begin{equation}
   \max_{\boldsymbol{x}} \sqrt{\boldsymbol{x}^T (\boldsymbol{X}^T \boldsymbol{X})^{-1} \boldsymbol{x} } \leq \frac{B(p)}{N^{\beta(p)}},
\end{equation}
\begin{table}[htbp]
  \centering
  \caption{$B(p)$ and $\beta(p)$}
    \begin{tabular}{ccccccccc}
    \toprule
    $p$     & 1     & 2     & 3     & 4     & 5     & 6     & 7     & 8 \\
    \midrule
    $\beta(p)$  & 0.08  & 0.08  & 0.18  & 0.29  & 0.45  & 0.75  & 1.21  & 1.82 \\
    $B(p)$     & 1.06  & 1.09  & 1.39  & 2.04  & 3.57  & 9.13  & 37.38 & 248.7 \\
    \bottomrule
    \end{tabular}%
  \label{tab: beta and c}%
\end{table}%

where $C(p)$ and $\beta(p)$ can be found in Table.~\ref{tab: beta and c}. Putting the results in \textbf{(1)} and \textbf{(2)} together and adding the subscript $\fs$ for Q functions and the parameter $K_\fs$, one can derive:
\begin{equation}
\label{equ: results for bounded error}
    ||\hat{Q}_\fs(s, a|\epsilon) - Q_\fs^*(s, a|\epsilon)|| \leq \frac{B(p) z_{\alpha/2}}{N^{\beta(p)}} \sqrt{ \sigma^2 \ M K_\fs^2},
\end{equation}
which is claimed in~(\ref{equ: bounded safety violation}).
\end{proof}

\subsection{Proof of Proposition~\ref{proposition: bounded safety violation}}
\label{proof: bounded safety violation}
\begin{proof}
With the definition of the versatile safe RL, the optimal policy $\pi^*$ should satisfy the constraint:
\begin{equation}
    V_c^{\pi^*(\mu_0|\epsilon)} \leq \epsilon,
\end{equation}
Consequently, with confidence $1-\alpha$:
\begin{equation}
\begin{aligned}
  V_c^{\pi(\mu_0|\epsilon)} - \epsilon & \leq V_c^{\pi(\mu_0|\epsilon)} - V_c^{\pi^*(\mu_0|\epsilon)} \\
  & = \E_{s_0 \sim \mu_0, a \sim \pi(\cdot | \epsilon)} \left[ Q_c(s, a|\epsilon) - Q_c^*(s, a|\epsilon) \right] \\
  & \leq \max_{(s, a)} Q_c(s, a|\epsilon) - Q_c^*(s, a|\epsilon) \\
  & \leq \frac{z_{\alpha/2} B(p)}{N^{\beta(p)}}  \sqrt{ \sigma^2 K_\fs^2 M },
  % \vspace{-5p}
\end{aligned}
\end{equation}
where the last inequality comes from Theorem~\ref{Theorem: Bounded estimation error}.
\end{proof}

% \subsection{Proof of the E-step objective (\ref{eq:estep_objective})}

\subsection{Proof of the closed-form solution (\ref{eq:optimalq_theorem})}
The closed-form solution is mainly derived from the EM-style safe RL training framework, and more details could be found in Appendix A.2 in~\cite{liu2022constrained}. For self-contained, we briefly introduce them as follows.
\label{app_subsection: Proof of the closed-form solution}
\begin{proof}
It should be noticed that we have an inherent constraint for $q(\cdot |s, \epsilon_i )$ to be a valid distribution:
\begin{equation}
    \int q(a | s, \epsilon_i) da = 1, \quad \forall s \sim \rho_q
\end{equation}

Then to solve the constrained optimization problem, we first convert it to the equivalent Lagrangian function:
\begin{align}
    L(q,\lambda, \eta, \kappa) & = \int \rho_q(s) \int q(a|s) \hat{Q}^{\pi_{\theta_j}}_r(s,a|\epsilon_i) da ds \\
    &+ \lambda \left( \epsilon_i - \int\rho_q(s)\int q(a|s, \epsilon_i) \hat{Q}^{\pi_{\theta_j}}_c(s,a|\epsilon_i) dads \right) \\ 
    & + \eta \left(\kappa - \int\rho_q(s)\int q(a|s, \epsilon_i) \log \frac{q(a|s, \epsilon_i)}{\pi(a|s, \epsilon_i)}dads \right) \\
    &+ \kappa \left(1 - \int\rho_q(s)\int q(a|s, \epsilon_i)dads \right),
    \label{eq:lagrangian}
\end{align}
where $\lambda, \eta, \kappa$ are the Lagrange multipliers for the constraints. 
Since the objective is linear and all constraints are convex (note that KL is convex), the E-step optimization problem is convex.
Then we obtain the equivalent dual problem:
\begin{equation}
    \min_{\lambda, \eta, \kappa} \max_{q(\cdot | \epsilon_i)} L(q(\cdot | \epsilon_i), \lambda, \eta, \kappa).
    \label{eq:dual_formulation}
\end{equation}

Take the derivative of the Lagrangian function w.r.t $q$:
\begin{equation}
    \frac{\partial L}{\partial q(\cdot | \epsilon_i)} = \hat{Q}^{\pi_{\theta_j}}_r(s,a| \epsilon_i) - \lambda \hat{Q}^{\pi_{\theta_j}}_c(s,a| \epsilon_i) - \eta - \kappa - \eta\log\frac{q(a|s, \epsilon_i)}{\pi(a|s, \epsilon_i)}.
    \label{eq:q_partial}
\end{equation}

Let (\ref{eq:q_partial}) be zero, then we have the form of the optimal $q$ distribution:
\begin{align}
    q^*(a|s, \epsilon_i) = {\pi_{\theta_j}}(a|s, \epsilon_i) \exp\left(\frac{\hat{Q}_r(s,a|\epsilon_i) - \lambda \hat{Q}_c(s,a|\epsilon_i)}{\eta}\right) \exp\left(-\frac{\eta+\kappa}{\eta}\right),
    \label{eq:optimalq}
\end{align}
where $\exp\left(-\frac{\eta+\kappa}{\eta}\right)$ could be viewed as a normalizer for $q(a|s, \epsilon_i)$ since it is a constant that is independent of $q(\cdot | \epsilon_i)$. Thus, we obtain the following form of the normalizer by integrating the optimal $q(\cdot | \epsilon_i)$:
\begin{align}
    \exp\left(\frac{\eta+\kappa}{\eta}\right) = \int \pi_{\theta_j}(a|s, \epsilon_i) \exp\left(\frac{Q_r^{\pi_{\theta_j}}(s,a|\epsilon_i) - \lambda Q_c^{\pi_{\theta_j}}(s,a|\epsilon_i)}{\eta}\right) da,
    \label{eq:normalizer}
\end{align}
\begin{align}
    \frac{\eta+\kappa}{\eta} = \log\int {\pi_{\theta_j}}(a|s, \epsilon_i) \exp\left(\frac{\hat{Q}^{\pi_{\theta_j}}_r(s,a | \epsilon_i) - \lambda \hat{Q}^{\pi_{\theta_j}}_c(s,a| \epsilon_i)}{\eta}\right) da.
    \label{eq:normalizer2}
\end{align}
Take the optimal $q$ distribution in Equation~(\ref{eq:optimalq}) and $\frac{\eta+\kappa}{\eta}$ in Equation~(\ref{eq:normalizer2}) back to the Lagrangian function~(\ref{eq:lagrangian}), we can find that most of the terms are cancelled out, and obtain the dual function $g(\eta, \lambda)$,
\begin{align}
    g(\eta, \lambda) = \lambda \epsilon_i + \eta \kappa + \eta \int \rho_q(s) \log \int \pi(a|s, \epsilon_i) \exp\left(\frac{\hat{Q}^{\pi_{\theta_j}}_r(s,a | \epsilon_i) - \lambda \hat{Q}^{\pi_{\theta_j}}_c(s,a | \epsilon_i)}{\eta}\right) da ds.
    \label{eq:dual}
\end{align}
The optimal dual variables are calculated by
\begin{align}
   \eta^*, \lambda^* = \arg\min_{\eta, \lambda} g(\eta, \lambda).
\label{eq:optimal_dual}
\end{align}
\end{proof}
A good property is that the dual function (\ref{eq:optimal_dual}) is convex (as revealed in appendix A.3 of~\cite{liu2022constrained}), so we could use off-the-shelf convex optimization tools to solve the dual problem.
