# Supplementary material for: Constraint-Conditioned Policy Optimization for Versatile Safe Reinforcement Learning
Source: arXiv:2310.03718 source file (2024-04-29)
Supplement: Supplementary file 6 [file more_baseline.tex]

% Table generated by Excel2LaTeX from sheet 'Sheet1'
\begin{table}[htbp]
  \centering
  \caption{\small C-CPO baseline comparison}
  \scriptsize
    \begin{tabular}{cccccccc}
    \toprule
    Tasks & stats & BC    & CC    & DC    & DR    & AR    & Average \\
    \midrule
          & Avg. R & \textcolor[rgb]{ .2,  .2,  .2}{686.08 ± 2.58} & \textcolor[rgb]{ .2,  .2,  .2}{455.87 ± 1.51} & \textcolor[rgb]{ .2,  .2,  .2}{565.98 ± 5.71} & \textcolor[rgb]{ .2,  .2,  .2}{304.09 ± 32.17} & \textcolor[rgb]{ .2,  .2,  .2}{602.05 ± 1.66} & \textcolor[rgb]{ .2,  .2,  .2}{522.81} \\
    C-CPO & Avg. CV & \textcolor[rgb]{ .2,  .2,  .2}{1.77 ± 0.67} & \textcolor[rgb]{ .2,  .2,  .2}{4.50 ± 2.08} & \textcolor[rgb]{ .2,  .2,  .2}{6.32 ± 2.32} & \textcolor[rgb]{ .2,  .2,  .2}{11.82 ± 5.85} & \textcolor[rgb]{ .2,  .2,  .2}{2.19 ± 0.63} & \textcolor[rgb]{ .2,  .2,  .2}{6.6} \\
          & Avg. R-G & \textcolor[rgb]{ .2,  .2,  .2}{676.27 ± 2.32} & \textcolor[rgb]{ .2,  .2,  .2}{454.62 ± 1.97} & \textcolor[rgb]{ .2,  .2,  .2}{559.71 ± 7.32} & \textcolor[rgb]{ .2,  .2,  .2}{300.85 ± 32.41} & \textcolor[rgb]{ .2,  .2,  .2}{592.89 ± 2.68} & \textcolor[rgb]{ .2,  .2,  .2}{516.87} \\
          & Avg. CV-G & \textcolor[rgb]{ .2,  .2,  .2}{2.09 ± 0.59} & \textcolor[rgb]{ .2,  .2,  .2}{4.94 ± 2.37} & \textcolor[rgb]{ .2,  .2,  .2}{6.75 ± 2.47} & \textcolor[rgb]{ .2,  .2,  .2}{13.07 ± 5.44} & \textcolor[rgb]{ .2,  .2,  .2}{2.28 ± 0.73} & \textcolor[rgb]{ .2,  .2,  .2}{5.83} \\
    \midrule
          & Avg. R & \textcolor[rgb]{ .2,  .2,  .2}{710.86 ± 20.47} & \textcolor[rgb]{ .2,  .2,  .2}{406.06 ± 6.30} & \textcolor[rgb]{ .2,  .2,  .2}{630.55 ± 40.03} & \textcolor[rgb]{ .2,  .2,  .2}{458.69 ± 12.98} & \textcolor[rgb]{ .2,  .2,  .2}{660.88 ± 4.82} & \textcolor[rgb]{ .173,  .227,  .29}{\textbf{573.41}} \\
    CCPO  & Avg. CV & \textcolor[rgb]{ .2,  .2,  .2}{0.59 ± 0.31} & \textcolor[rgb]{ .2,  .2,  .2}{1.60 ± 0.91} & \textcolor[rgb]{ .2,  .2,  .2}{0.32 ± 0.38} & \textcolor[rgb]{ .2,  .2,  .2}{0.23 ± 0.25} & \textcolor[rgb]{ .2,  .2,  .2}{3.13 ± 1.67} & \textcolor[rgb]{ .173,  .227,  .29}{\textbf{1.17}} \\
          & Avg. R-G & \textcolor[rgb]{ .2,  .2,  .2}{699.04 ± 20.48} & \textcolor[rgb]{ .2,  .2,  .2}{401.53 ± 5.59} & \textcolor[rgb]{ .2,  .2,  .2}{625.51 ± 40.12} & \textcolor[rgb]{ .2,  .2,  .2}{455.64 ± 11.83} & \textcolor[rgb]{ .2,  .2,  .2}{660.07 ± 5.26} & \textcolor[rgb]{ .173,  .227,  .29}{\textbf{568.36}} \\
          & Avg. CV-G & \textcolor[rgb]{ .2,  .2,  .2}{0.83 ± 0.42} & \textcolor[rgb]{ .2,  .2,  .2}{1.49 ± 0.38} & \textcolor[rgb]{ .2,  .2,  .2}{0.47 ± 0.55} & \textcolor[rgb]{ .2,  .2,  .2}{0.33 ± 0.37} & \textcolor[rgb]{ .2,  .2,  .2}{3.25 ± 1.48} & \textcolor[rgb]{ .173,  .227,  .29}{\textbf{1.27}} \\
    \bottomrule
    \end{tabular}%
  \label{tab: CPO baseline}%
\end{table}%
