# Supplementary material for: Constraint-Conditioned Policy Optimization for Versatile Safe Reinforcement Learning
Source: arXiv:2310.03718 source file (2024-04-29)
Supplement: Supplementary file 7 [file appendix-beta.tex]

\begin{table}[htbp]
  \centering
  \caption{$B(p)$ and $\beta(p)$}
    \begin{tabular}{ccccccccc}
    \toprule
    $p$     & 1     & 2     & 3     & 4     & 5     & 6     & 7     & 8 \\
    \midrule
    $\beta(p)$  & 0.08  & 0.08  & 0.18  & 0.29  & 0.45  & 0.75  & 1.21  & 1.82 \\
    $B(p)$     & 1.06  & 1.09  & 1.39  & 2.04  & 3.57  & 9.13  & 37.38 & 248.7 \\
    \bottomrule
    \end{tabular}%
  \label{tab: beta and c}%
\end{table}%
